# Supplementary material for: A nonlinear bending theory for nematic LCE plates
Source: arXiv:2203.04010 source file (2022-03-08)
Supplement: Supplementary file 1 [file appendix.tex]

\section{Interne Notizen}
\subsection{Some old comments}

\begin{remark}[convex/non-convex]

Our arguments for proving Lemma \ref{L:recov_general:curved} rely on the assumptions of
\begin{itemize}
\item[(1)]
	$S$ begin a bounded convex domain,
\item[(2)]
	$S$ having a piece-wise $C^1$-boundary.
\end{itemize}
However, these conditions could be relaxed to
\begin{itemize}
\item[(1')]
	$S$ being a bounded Lipschitz domain,
\item[(2')]
	the existence of some relatively closed $\Sigma\subset \partial S$ of vanishing $\mathcal H^1$-measure, such that $\partial S$ is $C^1$ on $\partial S\setminus \Sigma$.
\end{itemize}
(Note that (2) implies (2') of course, but also (1) implies (1'), cf. \cite[Corollary 1.2.2.3]{grisvard1985elliptic})

This assumption relaxation would only have an impact on Lemma \ref{LemmaFinePropertiesOfSmoothisometries} and Lemma \ref{L:recov_general:curved}, as explained in the following.

First, Point \ref{ItemPatchesAndBoundaries} of Lemma \ref{LemmaFinePropertiesOfSmoothisometries} would fail in general.
(Only $\overline{\mathcal{L}_i}\cap \partial V \subset \overline{\partial V\cap S}$ would still hold for $i\in\{1,\ldots,k_{BC}\}$.)
Therefore, in the beginning of the proof of Lemma \ref{L:recov_general:curved}, we would need to assume without loss of generality that $M_\delta$ vanishes not only on some neighbourhood $U$ of $\overline{\partial V\cap S}$ but also $M_\delta=0$ on all of $[\Gamma(t);(N\circ \Gamma)(t)]$ if this line segment intersects $U$ (for any $t\in(0,T)$).
Because then, the constructions would still yield $\alpha$ and $g$ such that \eqref{EqElChalten} holds, even though it could not be deduced via \eqref{EqManasluChanged} and Lemma \ref{LemmaFinePropertiesOfSmoothisometries} \ref{ItemPatchesAndBoundaries} anymore.
(And even though, continuity of $f$ in the proof of Lemma \ref{L:recov_general:curved} would only be preserved for $t$ such that $[\Gamma(t);(N\circ\Gamma)(t)]\cap \supp M_\delta\neq \emptyset$.)

Note that assuming $\mathcal A_\delta=0$ on above-mentioned sets would be possible without loss of generality because of (1'), (2') and \cite[Proposition 14]{HornungFine}.
(It implies that these sets can be chosen with arbitrarily small measures. Thus, a density argument applies.)
\end{remark}\bigskip

We want to start proving Lemma \ref{L:recov_general:curved} by adapting constructions of.

\subsection{Calculus for ansatzes}
\begin{lemma}[Curved Case, \cite{SCHMIDT07}]
\label{LemmaKonvergenzKrummerStrain}
Let $V\subseteq \R^2$ be bounded and open.
Let
$
	y\in C^\infty(\overline{V},\R^3)\cap H^2_{\mathrm{iso}}(V,\R^3)
$,
$	D\in C^\infty(\overline{V}\times[-\tfrac12,\tfrac12],\R^3)$,
$	g_1,g_2,\alpha\in C^\infty(\overline{V},\R)$ and 
$	\delta\in\R$.
As abbreviations, we write $R:=R_y$, $b:=b$, $\II:=\II_y$ and $g := (g_1,g_2)^\top$.
For all $(x',x_3)\in V\times (-\tfrac12,\tfrac12)$ and $h>0$, we set
\begin{align*}
	y_h (x',x_3) :=& (1-h\delta)y(x')+hx_3 b(x')+\\
	& + hR(x')\begin{pmatrix}g(x')\\ \alpha(x')\end{pmatrix}+h^2 R(x') D(x',x_3)\\
	& + h^2x_3R(x')
	\begin{pmatrix}
		\II(x')g(x')-(\nabla'\alpha(x'))^\top
		\\
		0
	\end{pmatrix}.
\end{align*}

Then, we obtain the uniform convergence
\begin{align}
\label{EqStollentroll}
\frac{R^\top\nabla\!_hy_h -I}{h}&\rightarrow 
	\left(
	\begin{array}{c|c}
		\begin{matrix}
			-\delta I_{2\times 2} +
			(x_3+\alpha)\II+\nabla'g \\
			\cline{1-1} -g^\top \II+\nabla'\alpha
		\end{matrix} 
		&\partial_3 D+\begin{pmatrix}
				\II g-\nabla'\alpha^\top\\0
			\end{pmatrix}
	\end{array} 
	\right).
\end{align}
%and
%\begin{equation}
%\label{EqFernhachingen}
%\frac{(\nabla\!_hy_h )^\top\nabla\!_hy_h -I}{h}\rightarrow -2\delta I 
%	+ 2\kappa C\,e_3\otimes e_3
%	+ 2
%	\sym\left(
%	\begin{array}{c|c}
%		\begin{matrix}
%			(x_3+\alpha)\II+\nabla'g \\
%			\cline{1-1} \begin{array}{cc}0\quad&\quad 0\end{array}
%		\end{matrix} 
%		&\partial_3 D
%	\end{array} 
%	\right).
%\end{equation}
Furthermore
\begin{equation}
\label{EqLaubwolf}
\lim_{h\rightarrow 0 }\frac1h\big(\|y_h - y\|_{L^\infty}+\|\nabla\!_hy_h-R\|_{L^\infty}\big)<\infty.
\end{equation}
\end{lemma}

\begin{proof}
Straightforward calculations yield
\begin{align*}
\nabla\!_hy_h  = 
%& (1-h\delta)R+ \kappa\begin{pmatrix}
%h^2\delta x_3\nabla'b\,|\,hCb
%\end{pmatrix}
%\\
%& + h 
%\left( 
%\begin{array}{c|c}(1-h\delta)x_3 \nabla'b & R\partial_3 D \end{array}
%\right) 
%+ h \left(\begin{array}{c|c} \nabla'\left[R\begin{pmatrix}g\\ \alpha\end{pmatrix}\right]&R\begin{pmatrix}
%\II g-\nabla'\alpha^\top\\0
%\end{pmatrix}\end{array}\right)+
%\\
%& + h^2\nabla'(RD)\\
%& + h^2 x_3
%\left(\begin{array}{c|c}
%\nabla'
%\left[R
%\begin{pmatrix}
%\II g-\nabla'\alpha^\top\\0
%\end{pmatrix}
%\right]
%& \begin{array}{c}0\\0\\0 \end{array}
%\end{array}\right)
%\\
%=& R 
%+ h \left[
%	 -\delta R 
%	 + \left(\begin{array}{c|c}x_3 \nabla'b & R\partial_3D\end{array}\right)
%	 + \left(\begin{array}{c|c}
%	 		\nabla'\left[R\begin{pmatrix}g\\ \alpha\end{pmatrix}\right] &R\begin{pmatrix}
%\II g-\nabla'\alpha^\top\\0
%\end{pmatrix}
%	 \end{array} \right) 
%\right]  
%+
%\\
%& + h^2 
%\left(
%	\begin{array}
%		{c|c}-\delta x_3\nabla'b
%		+\nabla'(RD)
%		+x_3\nabla'
%\left[R
%\begin{pmatrix}
%\II g-\nabla'\alpha^\top\\0
%\end{pmatrix}
%\right]
%		&0
%	\end{array}
%\right)\\
R+ hT +O(h^2),
\end{align*}
where
\begin{equation*}
T = -\delta R+
\left(
	\begin{array}{c|c}
		x_3 \nabla'b+\nabla'
		\left[
			R\begin{pmatrix}g\\ \alpha\end{pmatrix}
		\right]
		&R\partial_3D +R
			\begin{pmatrix}
				\II g-\nabla'\alpha^\top\\0
			\end{pmatrix}
	\end{array}
\right) 
\in C^\infty(\overline V\times[-\tfrac12,\tfrac12],\R^{3\times 3})
\end{equation*}
and
$\|O(h^2)\|_{L^\infty} \leq C h^2
$
for some $C>0$ and all $0<h<1$. 
In particular, \eqref{EqLaubwolf} is proven.
Furthermore
\begin{equation*}
	\frac{R^\top\nabla\!_hy_h -I}{h} \rightarrow R^\top T \quad\text{ strongly in }L^\infty.
\end{equation*}
Note that the remaining statement \eqref{EqStollentroll} follows easily by using the new claim
\begin{align}\label{eq:claim:only:difficult:term}
	R^\top\nabla'\left[R\begin{pmatrix}g\\\alpha\end{pmatrix}\right]=\begin{pmatrix}\alpha \II+\nabla'g\\-g^\top \II+\nabla'\alpha\end{pmatrix}.
\end{align}

To prove this claim, we set $G:=(g_1,g_2,\alpha)^\top$ and start to calculate $(R^\top\nabla'[RG])_{k\lambda}$ for some arbitrary $k\in\{1,2,3\}$ and $\beta \in\{1,2\}$:
\begin{equation}\label{eq:first:expans:diffic:term}
\begin{aligned}
(R^\top\nabla'(RG))_{k\beta}
&=\sum_{i=1}^3R_{ik}\partial_\beta(RG)_i \\
&= \sum_{j=1}^3G_j \underbrace{\sum_{i=1}^3\big(R_{ik}(\partial_\beta R_{ij})\big)}_{=:P_{kj}^\beta} +\sum_{i,j=1}^3R_{ik}R_{ij}\partial_\beta G_j.
\end{aligned}
\end{equation}
The rightmost sum can be simplified to $\partial_\beta G_k$, by using the identity $R^\top R=I$.
But even using $\partial_\beta (R^\top R)=0$, we also obtain 
\begin{equation}\label{eq:dRTR:eq:zeor}
P_{kj}^\beta+P_{jk}^\beta=0,\quad \text{ for }j,k\in\{1,2,3\}
\end{equation}
We want to apply this to examine certain cases for the factor $P_{kj}^\beta$.
 
Case 1: In the case $j=k\in\{1,2,3\}$, we obtain from \eqref{eq:dRTR:eq:zeor} that $P_{kj}^\beta=0$.
%\begin{align*}
%	\sum_{i=1}^3R_{ik}(\partial_\beta R_{ij}) = 0.
%\end{align*}

Case 2:
In the case $j\neq k,\,\{j,k\}\subseteq\{1,2\},\,k=\beta$ we use Schwarz's theorem to obtain $\partial_\beta R_{ij} = \partial_\beta\partial_j y_i = \partial_jR_{i\beta}$ and hence
\begin{align*}
	P_{kj}^\beta = \sum_{i=1}^3 R_{ik}\partial_\beta R_{ij} &
	=\sum_{i=1}^3 R_{ik}\partial_j R_{i\beta}
	= P_{k\beta}^j 
	\stackrel{\text{Case 1}}{=}0.
\end{align*}

Case 3:
In the case $j\neq k,\,\{j,k\}\subseteq\{1,2\},\,j=\beta$ follows similarly as in Case 2 that
\begin{align*}
	P_{kj}^\beta
	&\stackrel{\eqref{eq:dRTR:eq:zeor}}{=} -P_{jk}^\beta
	= - P_{j\beta}^k
	\stackrel{\text{Case 1}}{=}0.
\end{align*}

Case 4: In the case $j\neq k,\,j=3$ follows by the definition of $\II$, that $P_{kj}^\beta = \II_{k\beta}$.

Case 5: In the case $j\neq k,\,k=3$ follows by Case 4 and \eqref{eq:dRTR:eq:zeor} that $P_{kj}^\beta = -\II_{j\beta}$.

From all these cases and \eqref{eq:first:expans:diffic:term}, we can finally conclude
\begin{align*}
	(R^\top\nabla'(RG))_{k\beta}
	& =\sum_{j=1}^3 P_{kj}^\beta G_j +\partial_\beta G_k = 
	\begin{cases}
		G_3\II_{k\beta}+\partial_\beta G_k &\text{ if }{k\neq 3},\\
		\sum_{j=1}^2G_j(-\II_{\beta j})+\partial_\beta G_k &\text{ if k = 3}.
	\end{cases}
\end{align*}
Written in matrix notation, and replacing $G$ by it's definition, the latter implies \eqref{eq:claim:only:difficult:term} and the proof is finished.
\end{proof}

\begin{lemma}[Flat Case, \cite{DPG20}]
\label{LemmaKonvergenzFlacherStrain}
Let $V\subseteq \R^2$ be bounded and open
and suppose that $y\in C^\infty(\overline{V},\R^3)\cap H^2_{\mathrm{iso}}(V,\R^3)$ satisfies $\II_y=0$ everywhere.
Furthermore, let $D\in C^\infty(\overline{V}\times[-\tfrac12,\tfrac12],\R^3)$, $w_1,w_2,v\in C^\infty(\overline{V},\R)$ and $\delta\in\R$.
As abbreviations, we write $\II:=\II_y$, $b:=b_y$, $R:=R_y$ and $w:=(w_1,w_2)^\top$.
For all $x=(x',x_3)\in V\times (-\tfrac12,\tfrac12)$ and $h>0$, we set
\begin{align*}
	y_h (x',x_3):= 
	& (1-h\delta)y(x') + h x_3 b(x') \\
	& + h \nabla'y(x')w(x')\\
	&+ h^2RD(x) + \sqrt{h} b(x')v(x')-h^\frac{3}{2} x_3 \nabla'y(x')\nabla'v(x')^\top\\
	& - \frac{1}{2}h^2x_3b(x')|\nabla'v(x')|^2.
\end{align*}

Then, we obtain
\begin{equation}\label{EqWaldspinnenhexe}
\lim_{h\rightarrow 0 } h^{-\frac12}\big(\|y_h - y\|_{L^\infty}+\|\nabla\!_hy_h-R\|_{L^\infty}\big)<\infty.
\end{equation}
and also the uniform convergence
\begin{equation*}
\frac{(\nabla\!_hy_h )^\top\nabla\!_h y_h  -I}{h}
 \rightarrow
\iota
\left(
-2\delta I_{2\times 2}
+
2\nabla_{sym}'w+\nabla'v^\top\otimes\nabla'v^\top 
\right)
 +2\sym{\partial_3D\otimes e_3}.
\end{equation*}
\end{lemma}

\begin{proof}
Straightforward calculations exploiting local constancy of $R$ (which comes from $\II = 0$) yield
\begin{equation*}
\nabla\!_hy_h =R+ \sqrt{h}R P_\frac{1}{2} + h R P_1 + h^\frac{3}{2}R P_{h,\frac{3}{2}},
\end{equation*}
where
\begin{align*}
		P_\frac{1}{2} 
	&
		=
		\left(\begin{array}{c|c}
				0
			&
				-\nabla'v^\top
			\\
			\cline{1-2}
				\nabla'v
			&
				0
		\end{array}\right),
	\\
		P_1 
	& 
		=  
		\left(\begin{array}{c|c}
				-\delta I_{2\times 2} +\nabla'w
			&
				\begin{array}{c}0\\0\end{array}
			\\
			\cline{1-2}
				\begin{array}{cc}0&0\end{array}
			&
				-\tfrac12 |\nabla'v|^2
		\end{array}\right)
		+\partial_3D\otimes e_3,
	\\
		P_{h,\frac{3}{2}} & = -
		\left(\begin{array}{c|c}
				x_3(\nabla')^2 v
			&
				\begin{array}{c}0\\0\end{array}
			\\
			\cline{1-2}
				\begin{array}{cc}0&0\end{array}
			&
				0
		\end{array}\right)
		+ \sqrt{h}
		\left(\begin{array}{c|c}
				\nabla'D 
			&
				\begin{matrix}0\\0\\0\end{matrix}
		\end{array}\right)
		- \frac{1}{2} \sqrt{h}x_3
		\left(\begin{array}{c|c}
				0
			&
				\begin{array}{c}0\\0\end{array}
			\\
			\cline{1-2}
				\nabla'(|\nabla'v|^2)
			&
				0
		\end{array}\right).
		.
\end{align*}
Because of the assumptions, we obtain some $C>0$ such that for all $h>0$ small enough
\begin{equation}\label{EqHalbmond}
	\|P_1\|_{L^\infty}\leq C,\quad \|P_\frac{1}{2}\|_{L^\infty}\leq C,\quad \|P_{h,\frac{3}{2}}\|\leq C.
\end{equation}
In particular \eqref{EqWaldspinnenhexe} is proven.

Now, we can calculate that
%\begin{equation}
%\label{eqZweiRinge}
%\begin{aligned}
%{\nabla\!_hy_h }^\top\nabla\!_hy_h 
%& = (R^\top+ \sqrt{h}P_\frac{1}{2}^\top R ^\top + h  P_1^\top R^\top  + h^\frac{3}{2}(P_{h,\frac{3}{2}})^\top R^\top ) (R+ \sqrt{h}R P_\frac{1}{2} + h R P_1 + h^\frac{3}{2}RP_{h,\frac{3}{2}})\\
%& = I + \sqrt{h}2\sym(P_\frac{1}{2}^\top )  +  h (2\sym(P_1^\top ) + P_\frac{1}{2}^\top P_\frac{1}{2}) + h^\frac{3}{2} Rest_h \\
%& = I   +  h (\underbrace{2\sym(P_1^\top ) + P_\frac{1}{2}^\top P_\frac{1}{2}}_{=:T}) + h^\frac{3}{2} Rest_h ,
%\end{aligned}
%\end{equation}
\begin{equation*}
%\label{eqZweiRinge}
{\nabla\!_hy_h }^\top\nabla\!_hy_h 
= I   +  h \left(2\sym(P_1^\top ) + P_\frac{1}{2}^\top P_\frac{1}{2}\right) + O\left(h^\frac{3}{2} \right),
\end{equation*}
where
%\begin{align*}
%Rest_h  = 
%& P_{h,\frac{3}{2}} +P_\frac{1}{2}^\top (P_1+\sqrt{h}P_{h,\frac{3}{2}}) + P_1^\top (P_\frac{1}{2}+\sqrt{h}P_1+ hP_{h,\frac{3}{2}})\\
%& + {P_{h,\frac{3}{2}}}^\top   (I+\sqrt{h}P_\frac{1}{2}+hP_1+h^\frac{3}{2}P_{h,\frac{3}{2}}),\\
%T =2\sym(P_1^\top ) + P_\frac{1}{2}^\top P_\frac{1}{2}
%& .
%\end{align*}
%and 
$\limsup_{h\rightarrow 0}h^{-\frac32}\|O(h^\frac32)\|_{L^\infty}<1$ because of \eqref{EqHalbmond}.
%Because of \eqref{EqHalbmond}, we obtain for some $C>0$ and all $h>0$ small enough
%\begin{equation}
%\label{eqAlphaOmega}
%\|Rest_h \|_{L^\infty}\leq C.
%\end{equation}
Therefore
\begin{equation*}
\frac{(\nabla\!_hy_h )^\top \nabla\!_h y_h  -I}{h} \rightarrow 2\sym(P_1^\top ) + P_\frac{1}{2}^\top P_\frac{1}{2}
\quad\text{ strongly in }L^\infty,
\end{equation*}
and writing out the right hand side yields the remaining claim.
%It only remains, to calculate $T$:
%\begin{align*}
%{T}
%& = 2\sym P_1+P_\frac{1}{2}^\top P_\frac{1}{2}\\
%& = -2\mathcal{C}I + 2\left(
%\begin{array}{c|c}
%\nabla_{sym}'w
%&
%\begin{matrix}
%0\\0
%\end{matrix}
%\\ \cline{1-2}
%\begin{matrix}
%0 & 0
%\end{matrix}
%& 
%0
%\end{array}
%\right) +2\sym{d\otimes e_3} -\left(
%\begin{array}{c|c}
%\begin{matrix}
%0&0\\0&0
%\end{matrix}
%&
%\begin{matrix}
%0\\0
%\end{matrix}
%\\ \cline{1-2}
%\begin{matrix}
%0 & 0
%\end{matrix}
%& 
%|\nabla'v|^2
%\end{array}
%\right)
% +2\kappa\delta\,e_3\otimes e_3\\
%&\quad + \left(
%\begin{array}{c|c}
%\nabla'v^\top \otimes\nabla'v^\top 
%&
%\begin{matrix}
%0\\0
%\end{matrix}
%\\ \cline{1-2}
%\begin{matrix}
%0 & 0
%\end{matrix}
%& 
%|\nabla'v|^2
%\end{array}
%\right)\\
%& = -2\mathcal{C}I + 2\left(
%\begin{array}{c|c}
%\nabla_{sym}'w
%&
%\begin{matrix}
%0\\0
%\end{matrix}
%\\ \cline{1-2}
%\begin{matrix}
%0 & 0
%\end{matrix}
%& 
%0
%\end{array}
%\right) +2\sym{d\otimes e_3} +2\kappa\delta\,e_3\otimes e_3\\
%&\quad + \left(
%\begin{array}{c|c}
%\nabla'v^\top \otimes\nabla'v^\top 
%&
%\begin{matrix}
%0\\0
%\end{matrix}
%\\ \cline{1-2}
%\begin{matrix}
%0 & 0
%\end{matrix}
%& 
%0
%\end{array}
%\right).
%\end{align*}
\end{proof}
